# Supplementary material for: LiDARDraft: Generating LiDAR Point Cloud from Versatile Inputs
Source: arXiv:2512.20105 source file (2026-07-29)
Supplement: Supplementary file 1 [file 7_X_suppl.tex]

\clearpage
\setcounter{page}{1}
\maketitlesupplementary
%KITTI360数据集每个场景序列都自带了布局文件，文件格式是xml，保存了每个物体的索引、类别、box顶点坐标、box转换到世界坐标系的变换矩阵、box出现和消失的帧序号等。首先，我们导入该xml文件筛选出“地面”，“树木”，“车辆”，“房屋”等类别，去除一些容易干扰的'unlabeled' 、'trash bin' 、'rail track'等类别，按照box顶点坐标和变换矩阵逐个加载物体到世界坐标系，构建如图1场景的全局布局。之后，借助Fresnel（https://fresnel.readthedocs.io/en/v0.13.7/）库的场景渲染功能，我们导入场景全局布局，根据自车轨迹设置相机轨迹，在BEV视角下可视化每一帧layout并观察自车轨迹。如下图2为Layout的BEV视角图，物体类别用不同的颜色区分开，每一种颜色对应一种语义，“树木”用绿色表示，“房屋”用黑色表示，“车辆”用蓝色表示，自车轨迹用白色线条表示。这样我们就得到了KITTI360数据集每一帧点云对应的布局，布局当作条件控制的输入，点云当作控制结果的真值，训练一个布局到点云的条件控制模型。
\section{Supplementary Material}
\section{A. Further Explanation of Concepts}
\subsection{Metrics}

We use the following metrics to evaluate the quality of generated point clouds, Jensen-Shannon Divergence(JSD), Minimum Matching Distance(MMD) and Frechet Range Distance(FRD).

\textbf{Jensen-Shannon Divergence(JSD)} measures the similarity between the probability distribution of synthesized and that of reference point clouds. Given the generated set $S$ and the reference set $R$ with probability density as $P_R$ and $P_S$ respectively, JSD is mathematically defined as follows: \begin{equation}
    \text{JSD}(P_S||P_R) = \frac{1}{2}D_{KL}(P_R || \frac{P_R+P_S}{2}) + \frac{1}{2}D_{KL}(P_S||M) 
\end{equation}where $D_{KL}$ is KL divergence. 

\textbf{Minimum Matching Distance(MMD)} indicates how close the generated point cloud set $S$ align with the reference set $R$. It is calculated as the average distance of the point pairs matched with minimum distance. Mathematically, it is defined as follows: 
\begin{equation}
    MMD(P_S||P_R)=\frac{1}{|P_R|} \sum\limits_{Y\in P_R} \min\limits_{X\in P_S} CD(X,Y) 
\end{equation}where $CD$ is Chamfer Distance.

\textbf{Frechet Range Distance(FRD)} serves as a perceptual metric for range image and thus evaluates the perceptual correctness of generated point clouds.  

\textbf{FPD} Leveraging the support of point clouds, the hybrid of point clouds and sparse volumes preserves a richer set of geometric information compared to utilizing sparse volumes alone. In the calculation of FPD, we employ SPVCNN~\cite{spvcnn} as the backbone, utilizing its public implementation. The computational process of FPD results in a 1536-channel global feature representation.

\subsection{KITTI-360 Layout}

Each scene sequence in the KITTI-360 dataset is accompanied by a layout file in XML format. This file contains information such as the index and category of each object, the coordinates of the bounding-box vertices, the transformation matrix that maps the bounding box to the world coordinate system, and the frame indices when the object appears and disappears. 

First, we import the XML file and filter the categories to include "ground", "trees", "vehicles", "houses", and other relevant objects, while removing distracting categories such as 'unlabeled', 'trash bin', and 'rail track'. Using the vertex coordinates of the boundary box and the transformation matrices, we load each object into the world coordinate system and construct the global layout of the scene, as shown in Figure 1.

Next, utilizing the scene rendering functionality of the Fresnel library \cite{Fresnel}, we import the global layout of the scene and set the camera trajectory according to the ego-vehicle's path. The layout of each frame is visualized from a bird's-eye view (BEV) perspective, allowing us to observe the ego-vehicle's trajectory. In the BEV view of the layout, as shown in Figure 2, different object categories are distinguished by different colors, with each color representing a specific semantic label: green for "trees", black for "houses", blue for "vehicles", and white for the ego-vehicle trajectory.

In this way, we obtain the corresponding layout for each point cloud frame in the KITTI-360 dataset. The layout is used as the conditional input, and the point cloud serves as the ground truth control result. We then train a conditional control model to map the layout to the point cloud.

\begin{figure}
\centering
\includegraphics[width=0.45\textwidth]{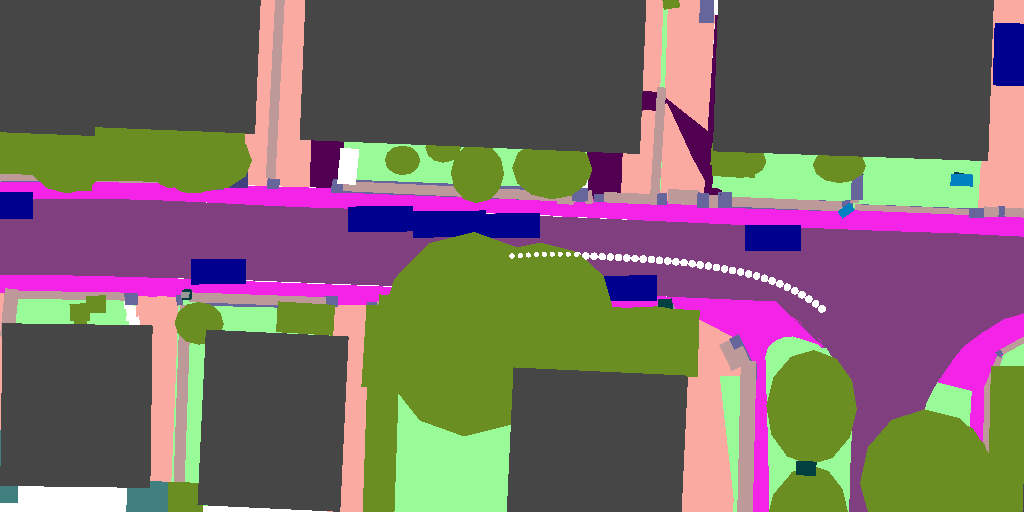}
\caption{The layout corresponding to a single frame of the KITTI-360 point cloud in the BEV view. Different object categories are distinguished by different colors.}
\label{fig:vegetation}
\end{figure}

\begin{figure}
\centering
\includegraphics[width=0.5\textwidth]{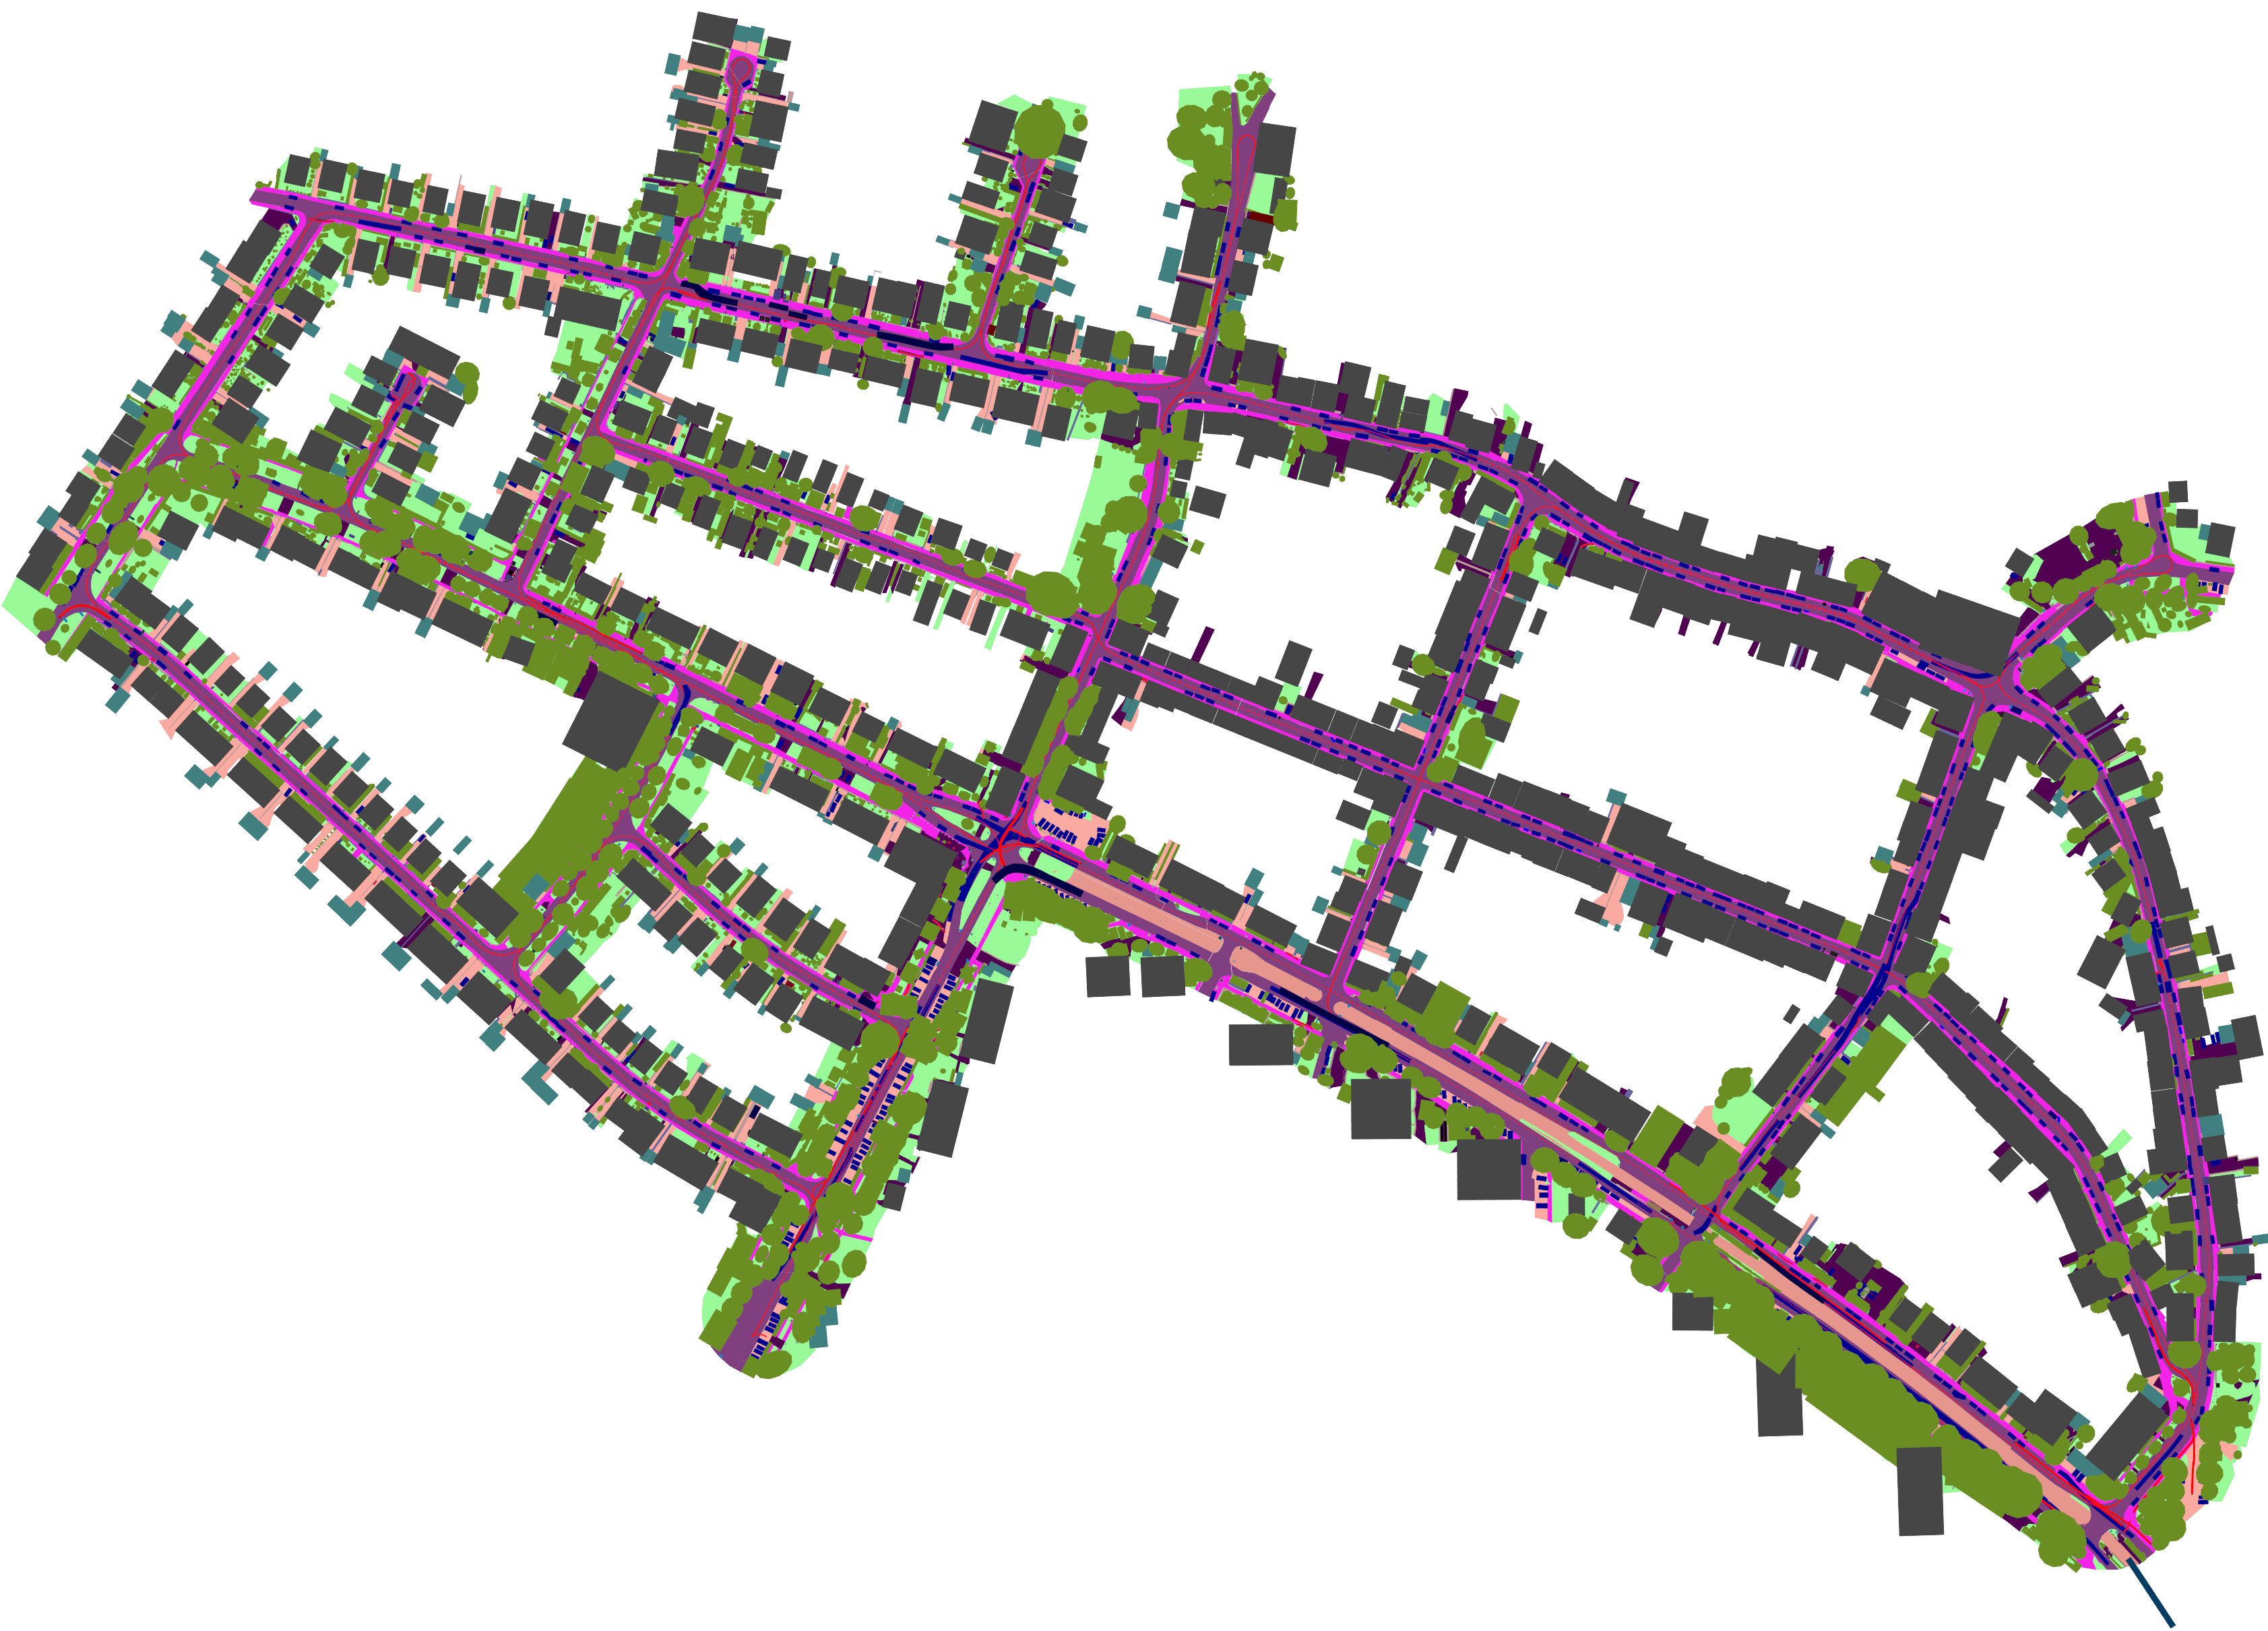}
\caption{The global layout of KITTI-360 sequence 0000.
}
\label{fig:globalview}
\end{figure}

\subsection{Raycasting}
%如上一节所述，我们得到了每帧点云及其对应的Layout，但是layout是3D网格形式，如何把点云和layout在数据类型上对齐是下一个需要解决的问题。关于layout和点云对齐方式，我们试过两种方法：表面均匀采样和raycasting，表面均匀采样是指在layout网格表面均匀采集点形成点云，raycasting是指从原点发射光线，计算光线和layout网格交点形成点云，如下图是两种方法形成layout的对比展示。具体来说，第一种表面均匀采样先设置lidar的局部坐标系位置，传感器采集范围，我们设置局部X坐标范围是[-80,80]，局部Y坐标范围是[-20,20]，由采集范围得到局部Layout后，在Layout表面均匀采集点构成点云。如下图直接在表面均匀采集的方式得到的点云虽然采集点很均匀，物体几何轮廓准确，但是无法反映物体之间的遮挡关系，只能给出物体布局粗略描述。实验发现，这种粗略描述是不够的，在训练layout条件控制点云模型时损失函数一直无法下降。第二种采用raycasting方法in Open3D，首先将雷达传感器的局部坐标系位置设置为原点，并根据激光雷达使用手册的FOV、角分辨信息设置发射光线，计算每一束光线和Layout网格三角片交点坐标，交点即为raycasting方法得到的点云。如下图，这种基于物理的方法不仅物体几何轮廓准确，采集点分布符合激光雷达沿圈扫描的传感特性，物体之间的空间遮挡关系也很好反映。所以我们最终采用raycasting方法将Layout网格转成和点云数据一致的类型。

As discussed in the previous section, we obtained the point clouds for each frame along with their corresponding layouts. However, the layout is in the form of a 3D grid, and aligning the point cloud with the layout in terms of data types is the next challenge we need to address. We explored two methods for aligning the layout and point clouds: uniform surface sampling and raycasting.

Uniform surface sampling refers to uniformly collecting points on the surface of the layout grid to form the point cloud, whereas raycasting involves emitting rays from an origin and calculating the intersection points between the rays and the layout grid to generate the point cloud. The following comparison illustrates the two methods for generating the layout.

Specifically, in the first method of uniform surface sampling, we first set the position of the LiDAR sensor's local coordinate system and the sensor's acquisition range. We set the local X-coordinate range to [-80, 80] and the local Y-coordinate range to [-20, 20]. Using this acquisition range, we generate the local layout and then uniformly sample points on the surface of the layout to form the point cloud. As shown in the figure, although the point cloud obtained by uniform surface sampling has evenly distributed points and accurate geometric contours of the objects, it does not reflect the occlusion relationships between objects and can only provide a rough description of the layout. Experimental results show that this rough description is insufficient, as the loss function does not decrease during the training of the layout-conditioned point cloud model.

The second method utilizes raycasting, implemented using Open3D. First, we set the local coordinate system of the LiDAR sensor to the origin and emit rays according to the sensor's field of view (FOV) and angular resolution, as described in the LiDAR manual. We calculate the intersection points between each ray and the layout grid's mesh triangles, with the intersection points forming the point cloud generated by the raycasting method. As shown in the figure, this physics-based method not only accurately captures the geometric contours of the objects but also produces point distributions that align with the scanning characteristics of the LiDAR sensor. Furthermore, the spatial occlusion relationships between objects are well represented. Therefore, we ultimately adopt the raycasting method to transform the layout grid into a format consistent with the point cloud data.

%然而，上述基于物理的raycasting模拟方法有点理想化，现实中由于lidar传感器噪声和误差、环境因素影响、自车运动速度变化都可能造成激光雷达光束掉落。 we 尝试使用一个 Stochastic Raydrop网络to simulate the noise typically observed in real-world LiDAR sampling, thereby generating the final LiDAR point cloud. 具体来说， we apply the Stochastic Raydrop approach, consistent with lidardm, which uses a real-world LiDAR scan Raydrop mask for supervision. Leveraging a U-Net architecture, we predict the Raydrop probability for each pixel in the input range map, addressing the issue of overly clean synthetic LiDAR data that does not sufficiently resemble real-world samples. Overall, through the integration of physics-informed ray casting and Stochastic Raydrop,可以得到一个更符合现实激光雷达传感器特性的数据。

However, the aforementioned physics-based raycasting simulation is somewhat idealized. In reality, noise and errors in LiDAR sensors, environmental factors, and variations in the ego-vehicle's speed can lead to laser beam dropouts. To address this, we attempt to simulate the noise typically observed in real-world LiDAR sampling by using a Stochastic Raydrop network to generate the final LiDAR point cloud. Specifically, we apply the Stochastic Raydrop approach, consistent with the LiDARDM framework, which uses a real-world LiDAR scan Raydrop mask for supervision. By leveraging a U-Net architecture, we predict the Raydrop probability for each pixel in the input range map, addressing the issue of overly clean synthetic LiDAR data that do not sufficiently resemble real-world LiDAR samples. Overall, through the integration of physics-informed raycasting and the Stochastic Raydrop approach, we obtain data that better reflects the characteristics of real-world LiDAR sensors.

\begin{figure}
\centering
\includegraphics[width=0.5\textwidth]{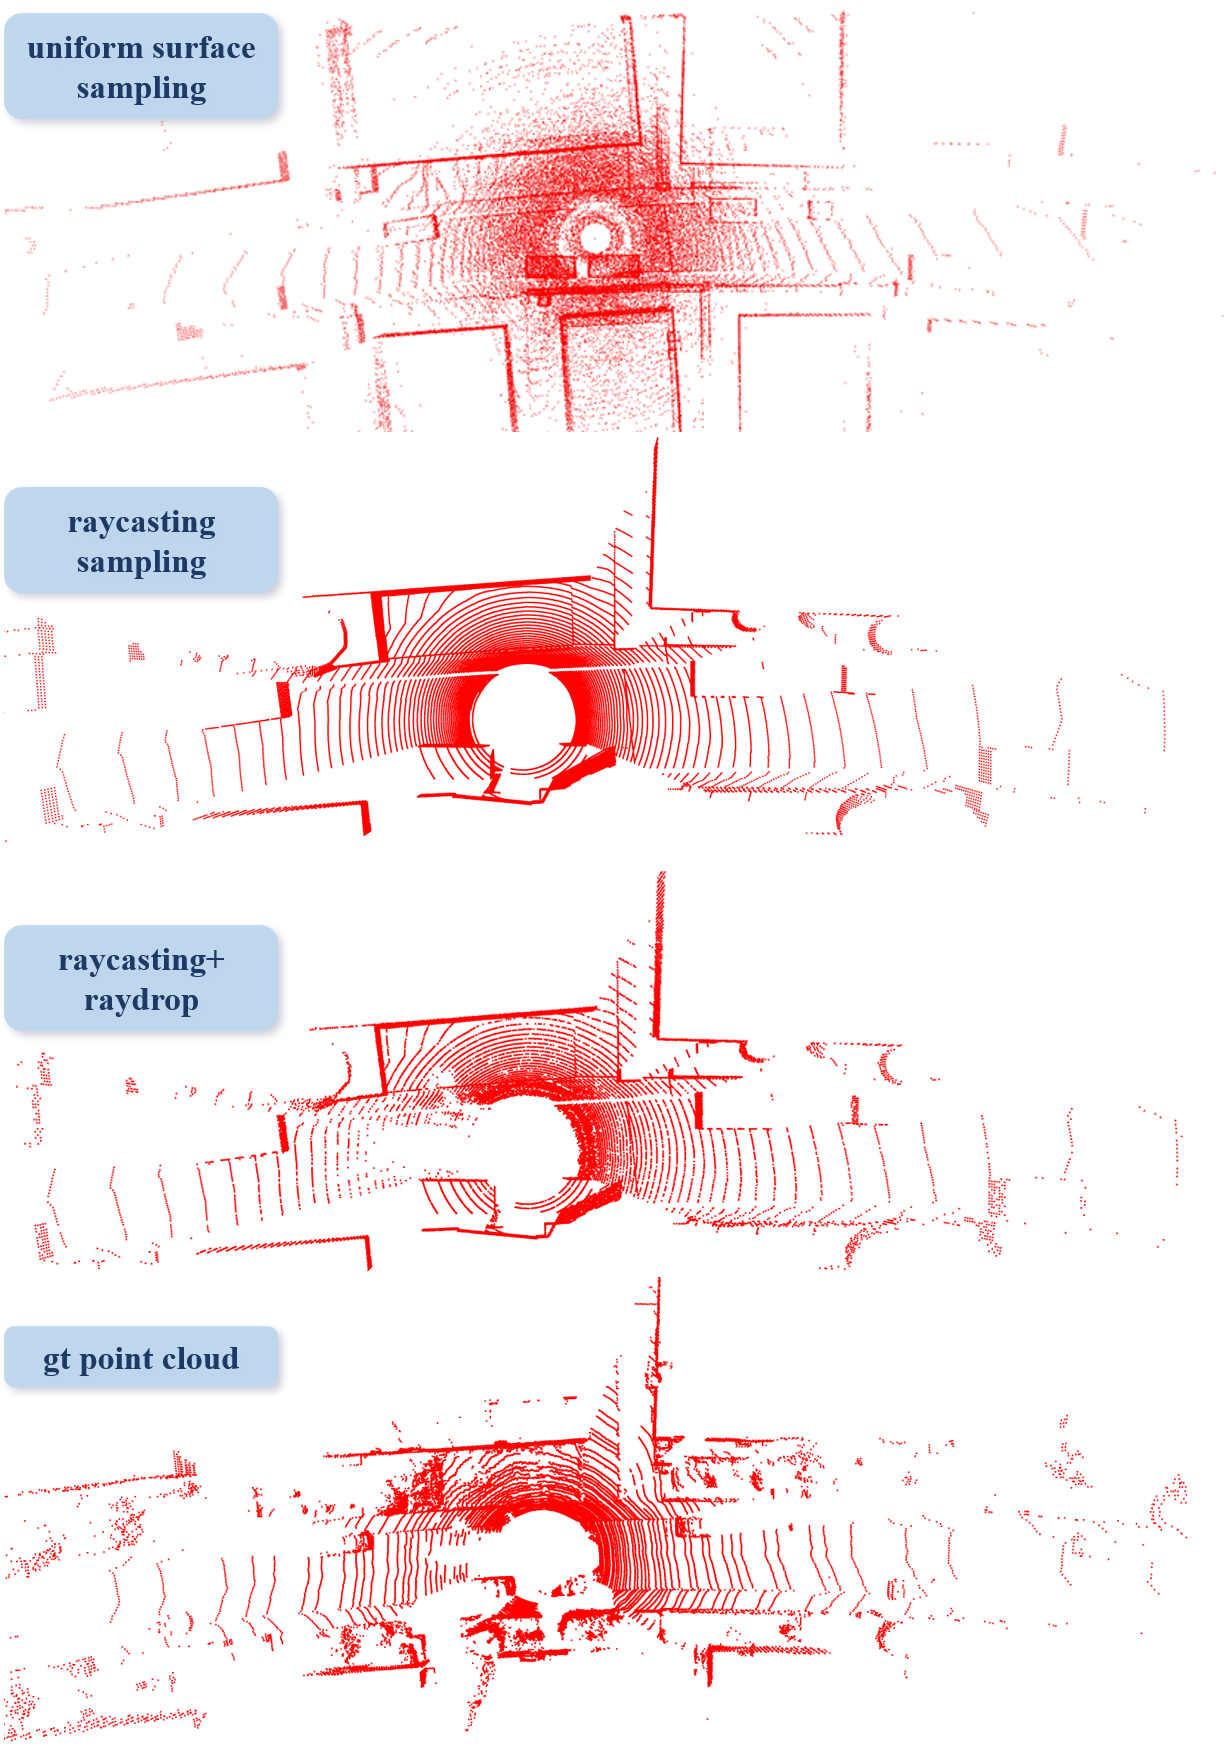}
\caption{The alignment of layout with different representations in point cloud space. 
From the first to the fourth row: (1) point cloud obtained by uniformly sampling the layout mesh surface, 
(2) point cloud generated by applying raycasting on the layout mesh, 
(3) point cloud processed by the RayDrop network after raycasting, 
and (4) the ground truth point cloud.
}
\label{fig:layout}
\end{figure}

%我们发现，上述raydrop网络在深度方面的确可以准确模拟出激光雷达的射线掉落，但由于原模型训练数据集语义标记和我们的语义标记不一致造成点云语义信息估计失败。如下图，使用了raydrop网络后，layout的语义信息不能正确区分类别，只有简单的有无交点信息。最后我们选择深度部分使用射线掉落网络而语义部分不使用射线掉落网络。
\begin{figure}[t]

\includegraphics[width=0.5\textwidth]{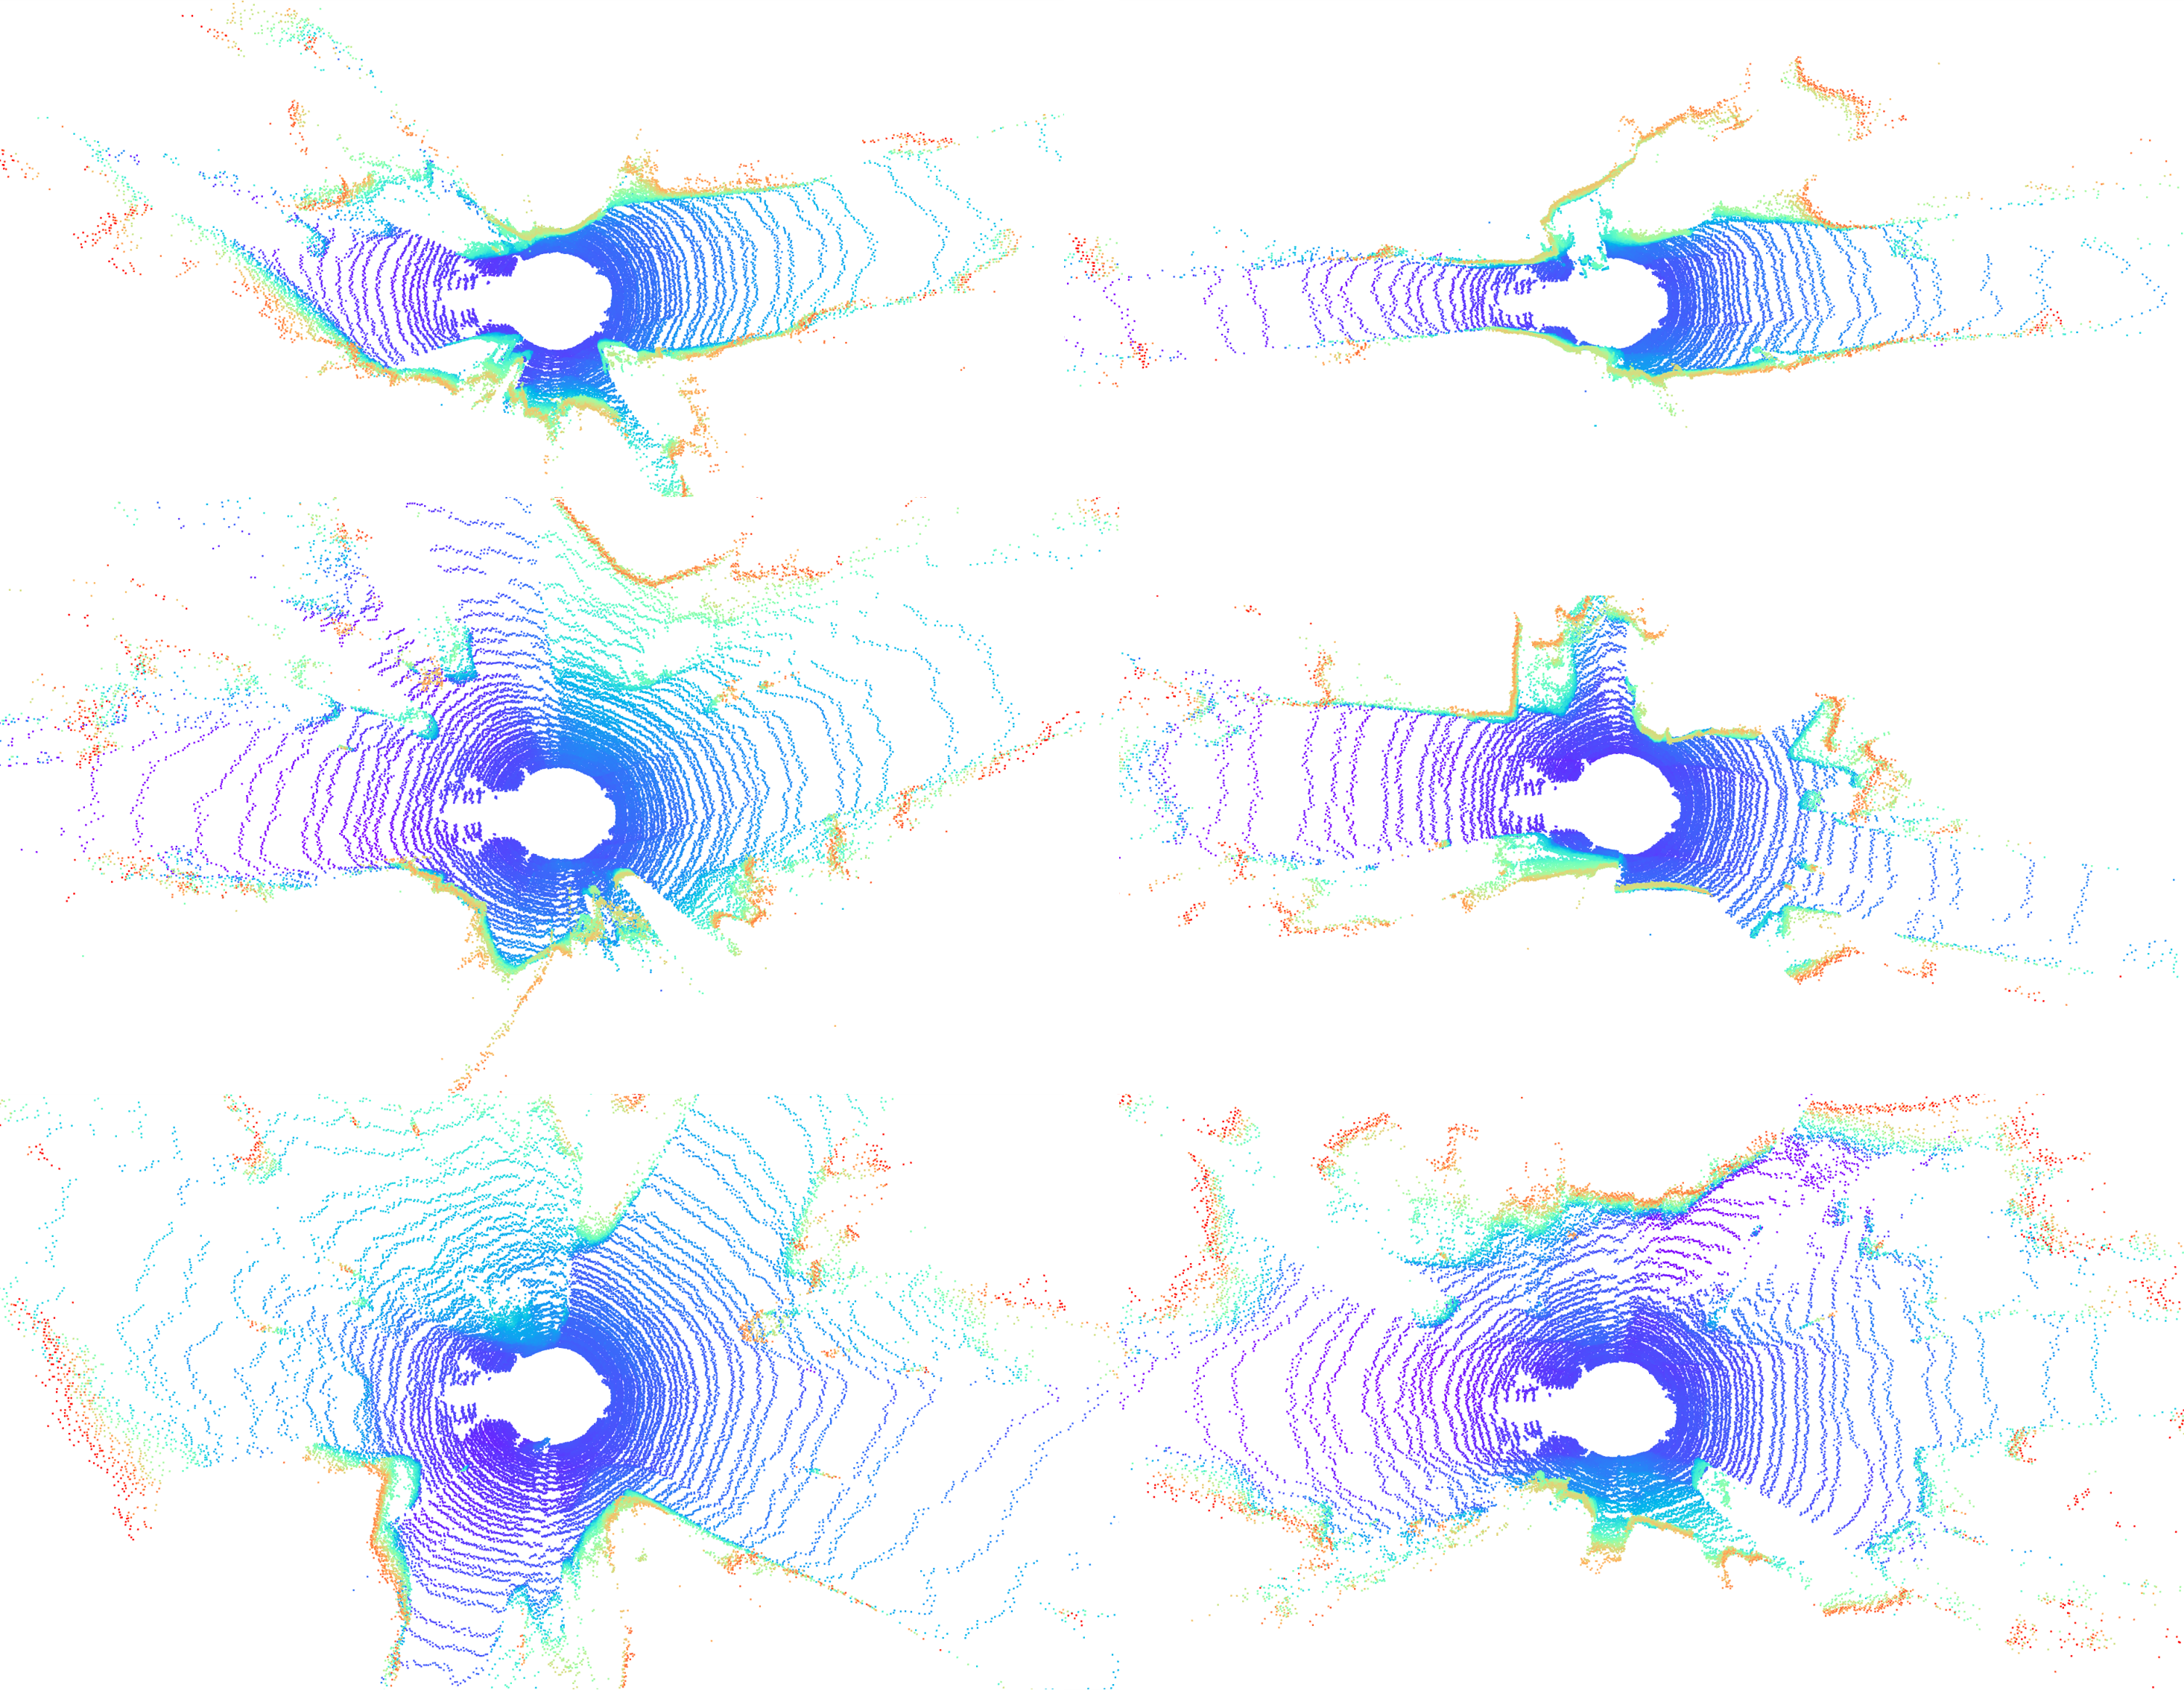}
\caption{Unconditional generation results of LiDAR-Draft, covering various driving scenarios, including straight roads, intersections, and vehicle turning conditions.
}
\label{fig:uncondiion}
\end{figure}

We found that although the Raydrop network accurately simulates LiDAR ray dropouts in terms of depth, the point cloud's semantic information estimation fails due to discrepancies between the semantic labels in the training dataset and our own semantic labeling. As shown in the figure, after applying the Raydrop network, the semantic information of the layout cannot correctly distinguish between categories, providing only basic intersection presence information. Ultimately, we choose to apply the Raydrop network to the depth part while excluding it from the semantic part.

\begin{figure*}
\centering
\includegraphics[width=1\textwidth]{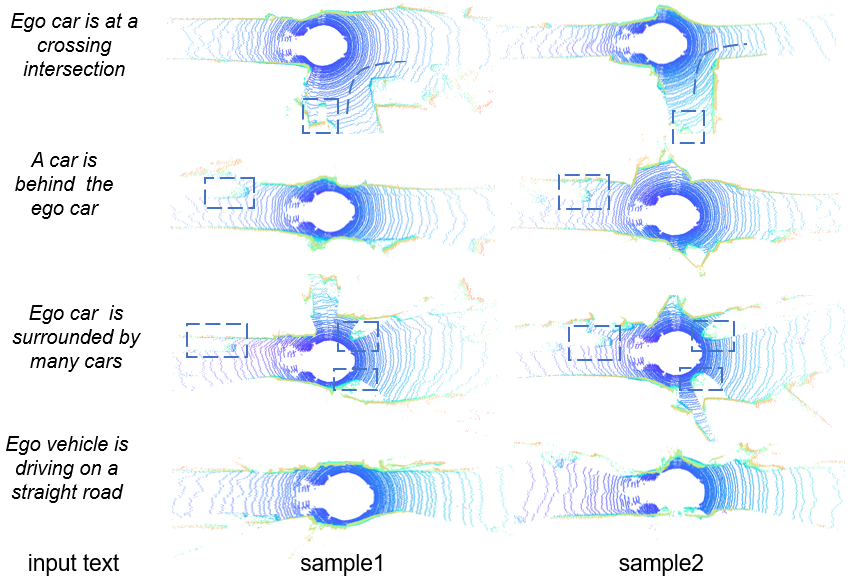}
\caption{Text-to-Point Cloud Generation Results: An automated driving scene layout description is generated with GPT and used to sample the point cloud. Blue boxes and lines highlight objects strongly aligned with the prompt.}
\label{fig:raydrop}
\end{figure*}

%我们的无条件生成基于lidarGen实现，lidargen将原始LiDAR点云转换为2.5维圆柱深度图，每一个像素对应激光雷达一条射线表示点云结构信息。使用Scored-based Energy Models输入W × H × 2 图像并输出相同大小( W × H × 2)得分图。我们先跟随Lidargen框架，重新训练了一个64线无条件生成模型，下图展示了我们64线无条件生成结果：结果图来看，无条件生成的点云连续平滑，道路交叉、车辆转弯、车辆遮挡都可以很好地生成。

\begin{figure}
\centering
\includegraphics[width=0.5\textwidth]{author-kit-CVPR2026-v1-latex-/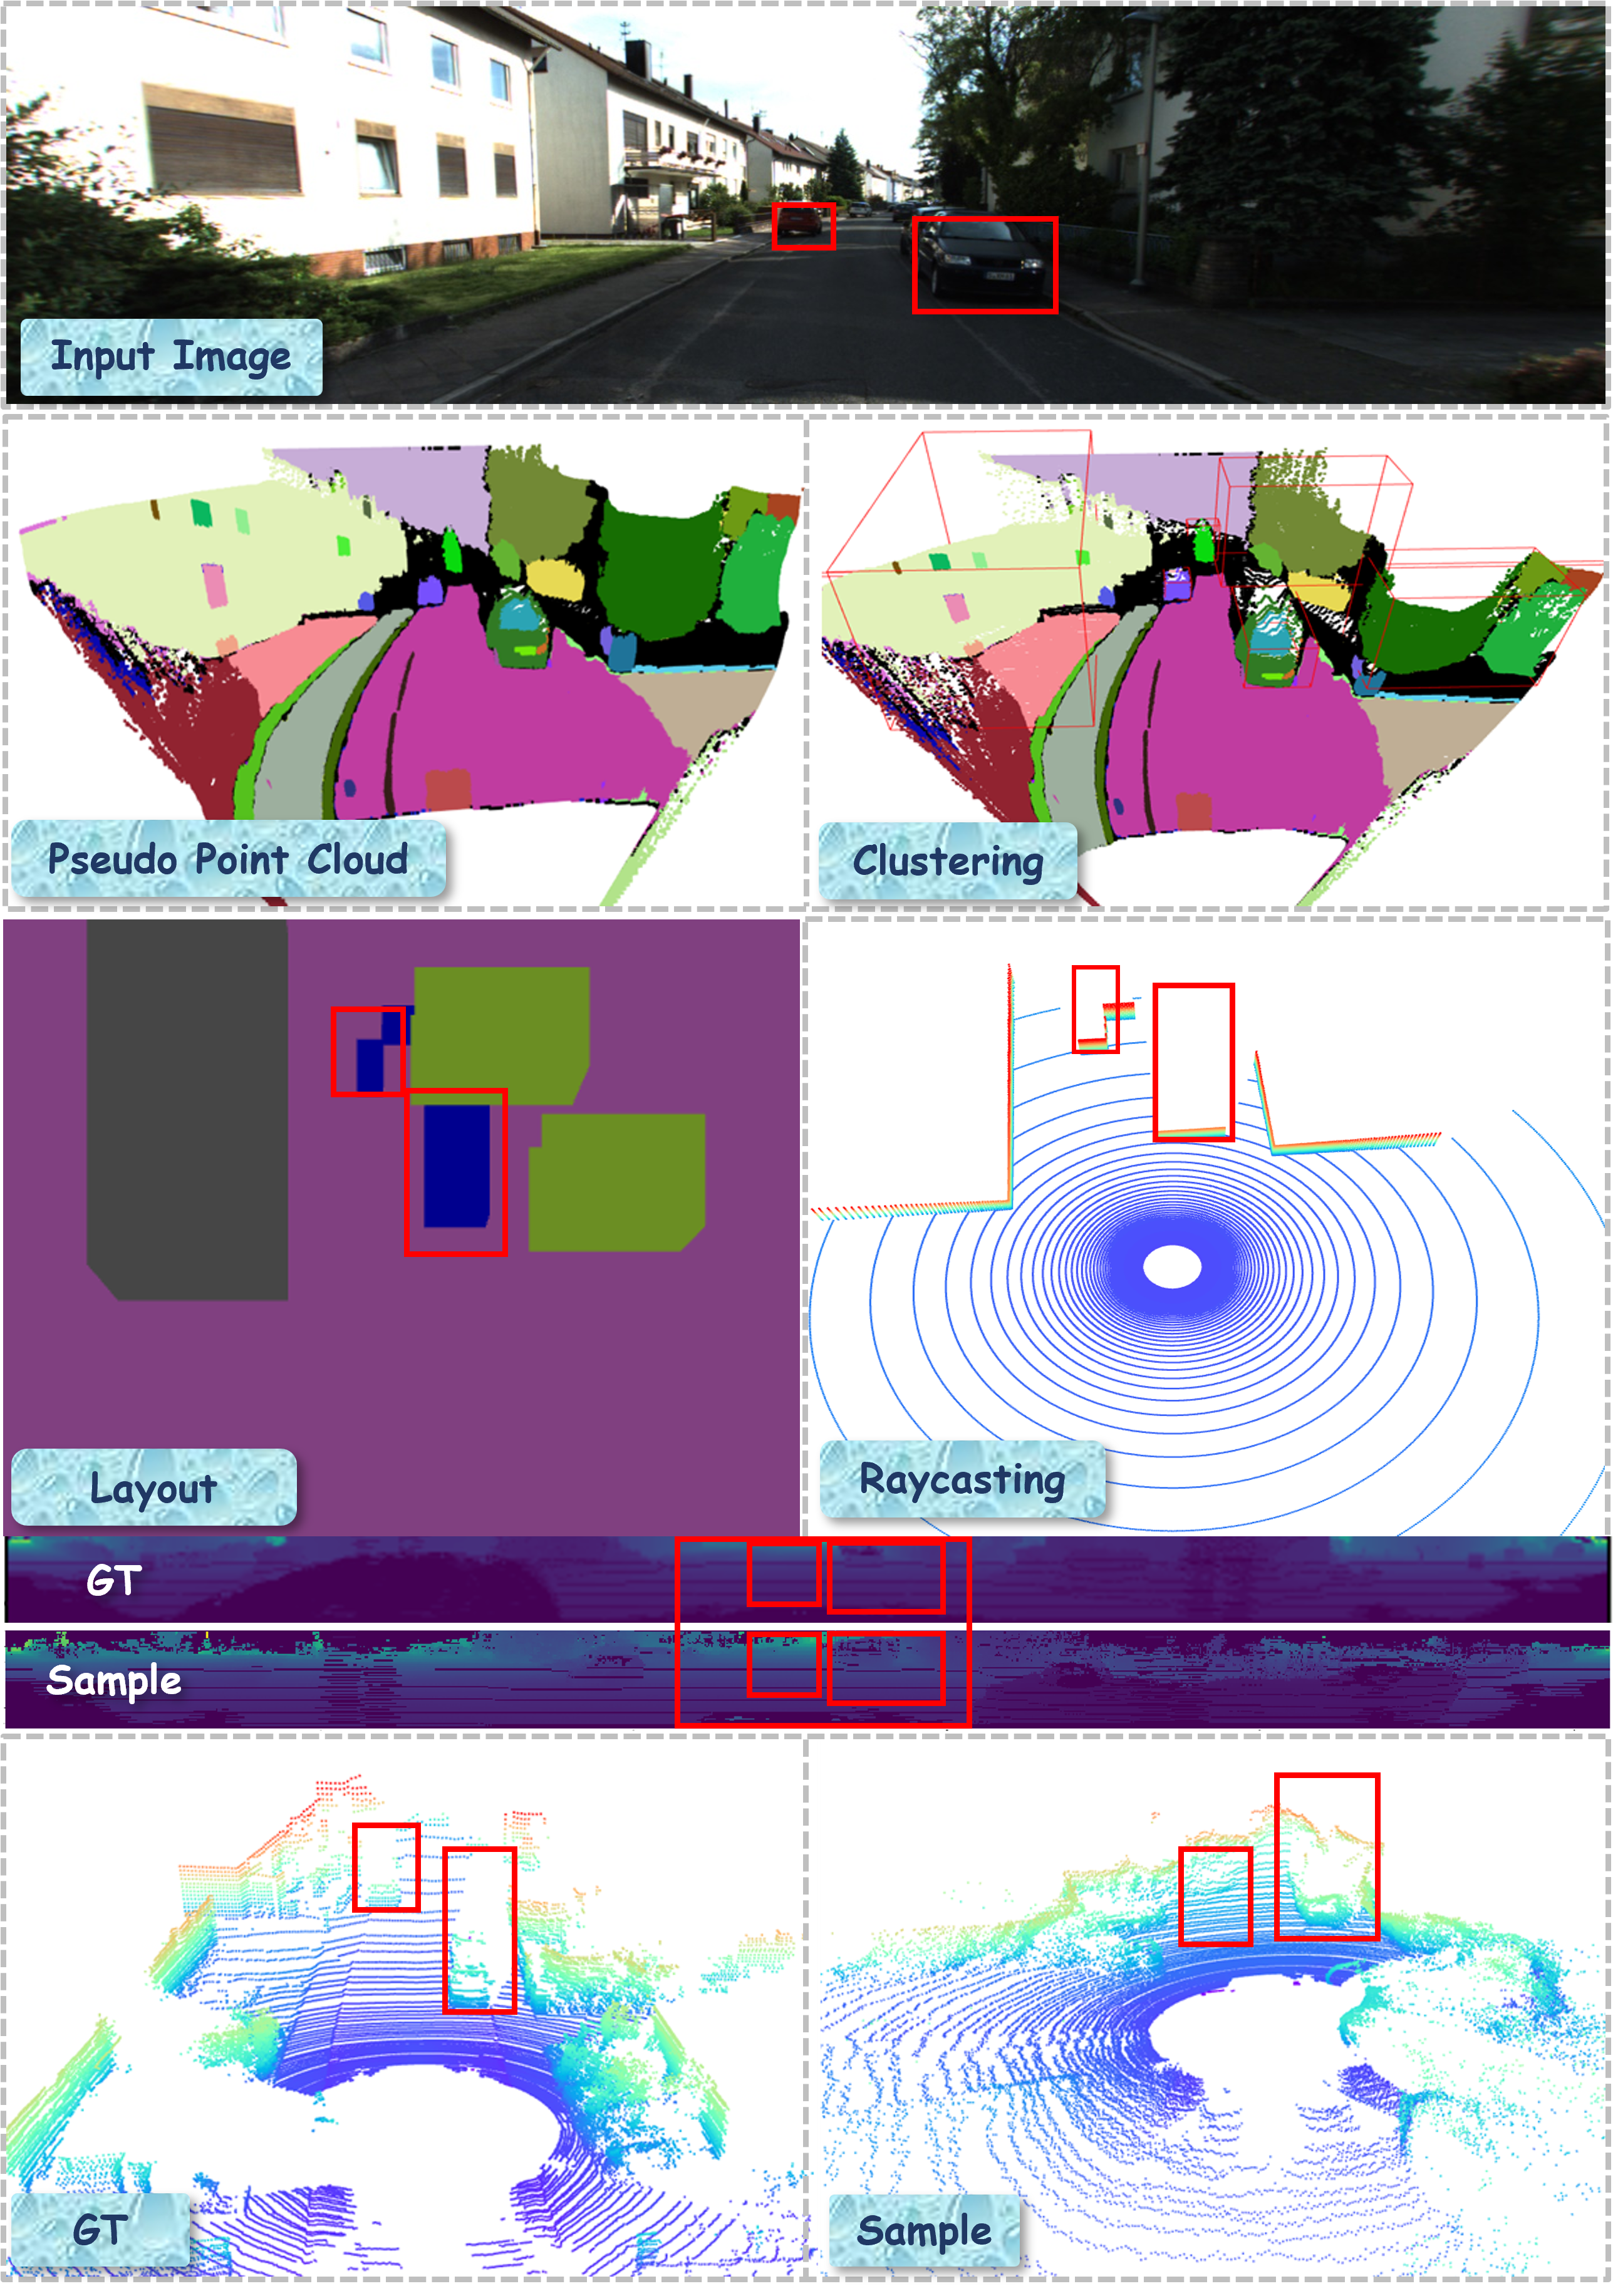}
\caption{The image-to-point cloud conditional generation process consists of the following steps: 
(1) Estimating the depth and semantics from the image, 
(2) Generating pseudo-point clouds from the semantics and depth, 
(3) Clustering the point clouds, 
(4) Constructing a layout from the clustering results, 
(5) Aligning the layout and point clouds using raycasting, 
(6) Generating point clouds from the layout 
(The figure compares the ground truth and sampled depth maps and 3D views.).
}
\label{fig:image2pcprocess}
\end{figure}

\section{B. Additional Experimental Results}
\subsection{Unconditional Generation}

Our unconditional generation is based on LiDARGen, which converts raw LiDAR point clouds into 2.5D cylindrical depth maps, where each pixel corresponds to a LiDAR ray and represents the structural information of the point cloud. We employ Score-based Energy Models (SBEMs) to take an input image of size \( W \times H \times 2 \) and output a score map of the same size \( (W \times H \times 2) \).

Following the LiDARGen framework, we retrained a 64-line unconditional generation model. The results of our 64-line unconditional generation are shown in the figure below. As observed, the generated point clouds exhibit smooth and continuous structures. Road intersections, vehicle turns, and occlusions between vehicles are effectively synthesized, demonstrating the model’s ability to generate high-quality LiDAR point clouds.

\subsection{Image to Point Cloud}
%如正文所述，图片和点云是自动驾驶相机和激光雷达两种传感器的主要模态，实现图片到点云条件控制生成有利于多模态的融合。正文介绍了我们图片到点云条件控制生成的框架：对图片进行语义分割和深度估计，用语义和深度投影成伪点云，伪点云聚类得到布局，再输入布局采样出点云。下面展示了生成过程：输入图片——投成伪点云——聚类——生成布局——射线投射——采样结果

As described in the main text, images and point clouds are the primary modalities captured by cameras and LiDAR sensors in autonomous driving. Achieving conditional generation from images to point clouds facilitates multi-modal fusion. The main text introduces our framework for the conditional image-to-point-cloud generation: we first perform semantic segmentation and depth estimation on the input image, then project the semantic and depth information to generate a pseudo point cloud. The pseudo point cloud is clustered to obtain the scene layout, which is subsequently used to sample the final point cloud. 

The generation process is illustrated as follows:  
\textbf{Input image} $\rightarrow$ \textbf{Pseudo point cloud projection} $\rightarrow$ \textbf{Clustering} $\rightarrow$ \textbf{Layout generation} $\rightarrow$ \textbf{Ray casting} $\rightarrow$ \textbf{Final sampled point cloud}.

%如正文所述，我们借助GPT-4和Blender实现文本到点云的条件控制生成，得到很好的效果。我们给GPT形如“请用blender帮我生成一个自车前放和左方各有一辆车的平直道路上，道路两旁都是树木vegetation，房屋building，房屋距离道路很近，树木距离道路也很近，但是不要互相干涉。物体颜色按照下面Label和RGB对应关系：Label(  'ground' , ( 81,  0, 81) ),Label(  'road' ，(128, 64,128) ), Label(  'building'，( 70, 70, 70) ), Label(  'car' , (  0,  0,142) ), Label(  'vegetation'  , (107,142, 35) )，大小按照真实尺寸，单位设置为米，比如road宽度按照双车道宽度7米，car、building也按照真实尺寸。同时生成一个自车搭载Velodyne HDL-64E传感器在这个场景中移动的轨迹吧，轨迹按照1*17矩阵的pose给出，中间空格隔开，第1个是帧序号，后面1*16是轨迹，轨迹数值也按照真实数据。”这样的描述要求GPT-4生成对应场景的python代码，并将代码导入blender生成layout场景。我们测试发现，GPT-4可以很好地理解道路类型（笔直道路、三岔路口、十字路口）、空间关系（前后）、尺寸大小（按照现实真实大小）等等，很容易地完成text描述生成3D layout任务，之后我们由layout采样点云，下面展示我们更多的生成结果：

\subsection{Text-to-Point Cloud Conditional Generation}

As described in the main text, we leverage GPT-4 and Blender to achieve conditional text-to-point cloud generation, yielding promising results. We provide GPT-4 with a prompt such as the following:

\textit{"Please use Blender to generate a straight road scene with one vehicle behind the ego vehicle. The road is lined with vegetation and buildings, both positioned close to the road without overlapping. The object colors should follow the Label-RGB mapping: Label('ground', (81, 0, 81)), Label('road', (128, 64, 128)), Label('building', (70, 70, 70)), Label('car', (0, 0, 142)), Label('vegetation', (107, 142, 35)). Object sizes should be realistic, with units in meters; for instance, the road width should be 7 meters (a two-lane road), and the sizes of cars and buildings should also follow real-world dimensions. Additionally, generate a trajectory for an ego vehicle equipped with a Velodyne HDL-64E sensor moving within this scene. The trajectory should be provided as a $1 \times 17$ matrix, where the first value represents the frame index, followed by a $1 \times 16$ trajectory matrix, separated by spaces, with values consistent with real-world data."}

GPT-4 then generates the corresponding Python code, which is imported into Blender to create the layout scene.

We conducted experiments and observed that GPT-4 can effectively comprehend different types of roads, including straight roads, T-junctions, and intersections. Below, we present additional generated results.

\subsection{Point Cloud Transformation}

Point cloud transformation is a common technique used to generate additional point clouds with layouts similar to the input, and is widely applied in data augmentation. In this work, the input point cloud is first segmented into different semantic categories. Then, DBSCAN clustering is applied to each category to generate bounding boxes (boxes). These boxes are combined to form a layout, which is subsequently used for sampling. The process is illustrated in the figure below:
Input Point Cloud → Semantic Segmentation → Clustering → Layout Generation → Ray Casting → Sampling Results.

\begin{figure}
\centering
\includegraphics[width=0.5\textwidth]{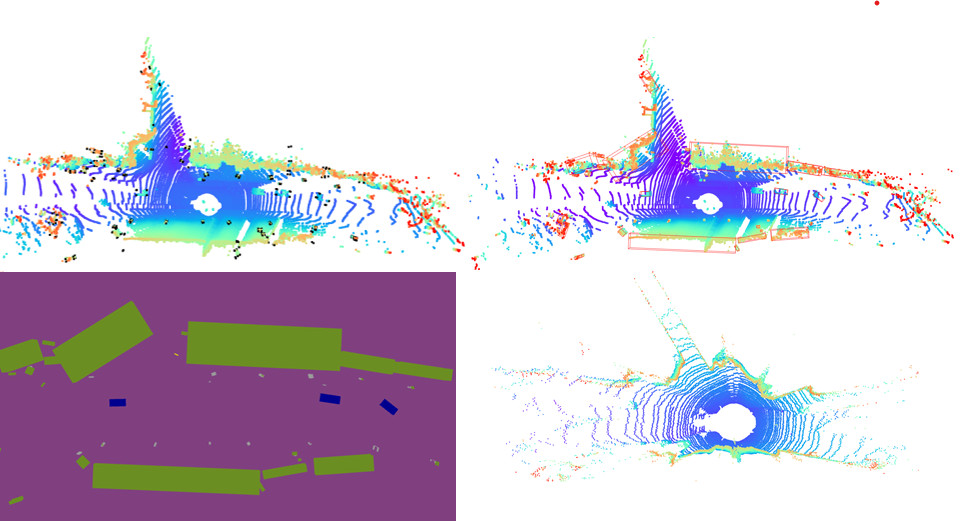}
\caption{The point cloud transformation process consists of the following steps: 
(1) Point cloud semantic segmentation, 
(2) Point cloud clustering, 
(3) Generating a layout from the clustering results, 
(4) Sampling point clouds from the layout.
}
\label{fig:pcprocess}
\end{figure}

\begin{figure}
\centering
\includegraphics[width=0.5\textwidth]{Figures/text2pc3.png}
\caption{Further text-to-point cloud conditional generation results are presented. The results demonstrate that LiDAR-Draft is able to effectively capture road types, spatial relationships, and quantitative relationships between objects.
}
\label{fig:text2pc3}
\end{figure}

\begin{figure*}
\centering
\includegraphics[width=1\textwidth]{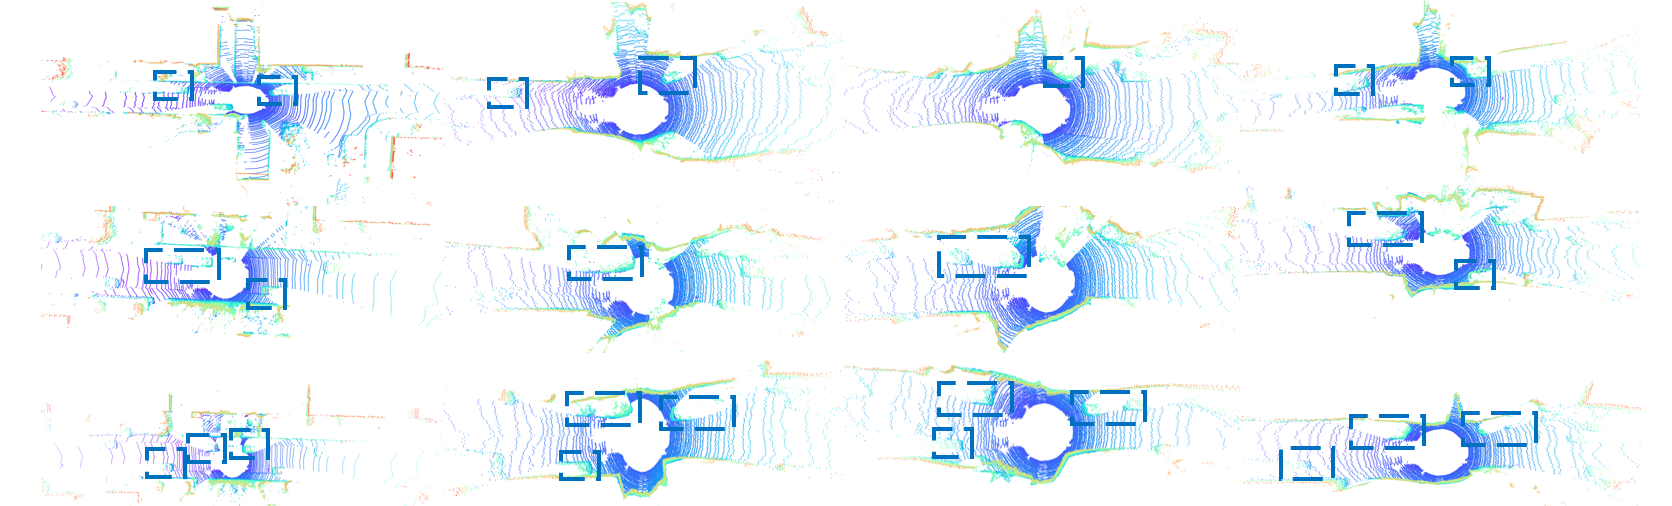}
\caption{Additional point cloud transformation results are presented. Given a single frame of the input point cloud, LiDAR-Draft is capable of generating multiple point clouds with consistent layouts, which contributes to enhancing the diversity of the point cloud data.
}
\label{fig:text2pc3}
\end{figure*}

\subsection{Multiple Input}

%lidardraft同时还支持多种类型输入，如图fig2，semantic/depth/semantic+depth都可以作为条件控制生成模型，并且具有相似的控制结果。如图fig9，无论是输入layout的语义还是深度信息，lidardraft都可以取得相似的控制效果。我们猜测这可能和整个框架都搭建在无条件点云生成上有关，由于数据处理、模型设计、训练方法都限制在无条件lidar点云生成上，可以保证采样结果是点云。这表明，lidardraft还能应用于缺少信息的layout场景。

The LiDARDraft framework supports multiple input types, as exhibited in \autoref{fig:semantic_vs_depth}, where semantic, depth, and semantic+depth information can serve as conditional controls for the generative model, achieving comparable control results. As illustrated in Fig. 9, LiDARDraft achieves consistent control effects regardless of whether the input layout consists of semantic or depth information. We hypothesize that this consistency stems from the fact that the entire framework is based on unconditional point cloud generation; data processing, model design, and training methods are all tailored to unconditional LiDAR point cloud generation, ensuring that the sampled outputs are point clouds. This capability suggests that LiDARDraft can also be effectively applied to layout scenarios where information may be missing.

\begin{figure}
\centering
\includegraphics[width=0.48\textwidth]{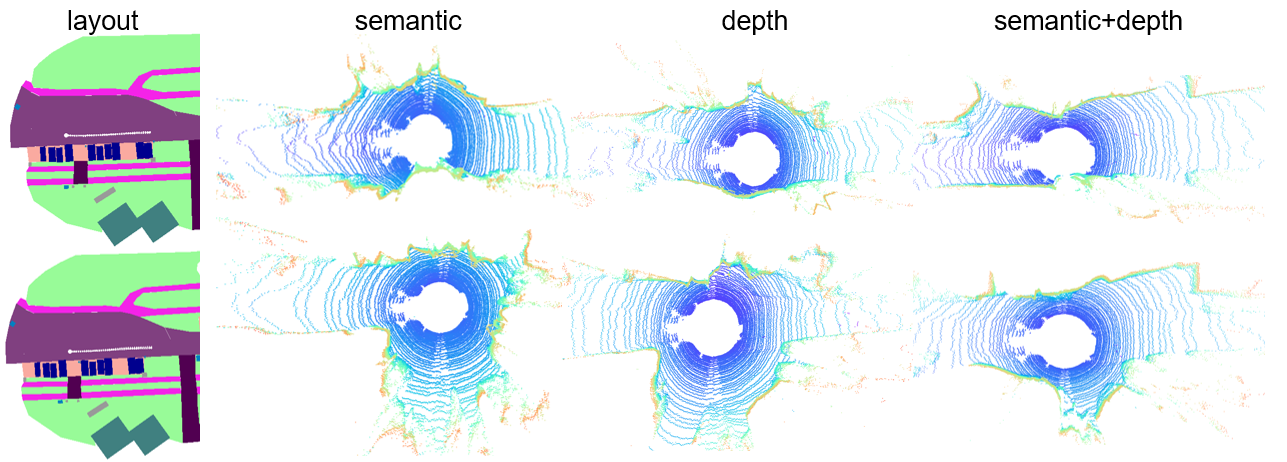}
\caption{LiDARDraft's Support for Language/Depth Input: Layouts with missing information can still control LiDAR point cloud generation. From left to right: the layout condition, point clouds generated with only semantic information in the layout, those with only depth information in the layout, and those with both semantic and depth information.}
\label{fig:semantic_vs_depth}
\end{figure}

\subsection{Semantic-KITTI Results}

We first trained an unconditional LiDAR point cloud generation model, LidarGen~\cite{lidargen}, on the KITTI-360~\cite{kitti360} dataset. Subsequently, we trained a conditional generation model on the SemanticKITTI~\cite{behley2019semantickitti} dataset to evaluate our model's cross-dataset performance. We found that the model successfully learned most of the dataset’s features within 2,000 fine-tuning steps, although certain finer details (e.g., car windows) were not fully captured at this stage. After 5,000 fine-tuning steps, however, the model effectively learned these finer details as well. More details are in the supplementary materials.
\begin{figure}
\centering
\includegraphics[width=0.48\textwidth]{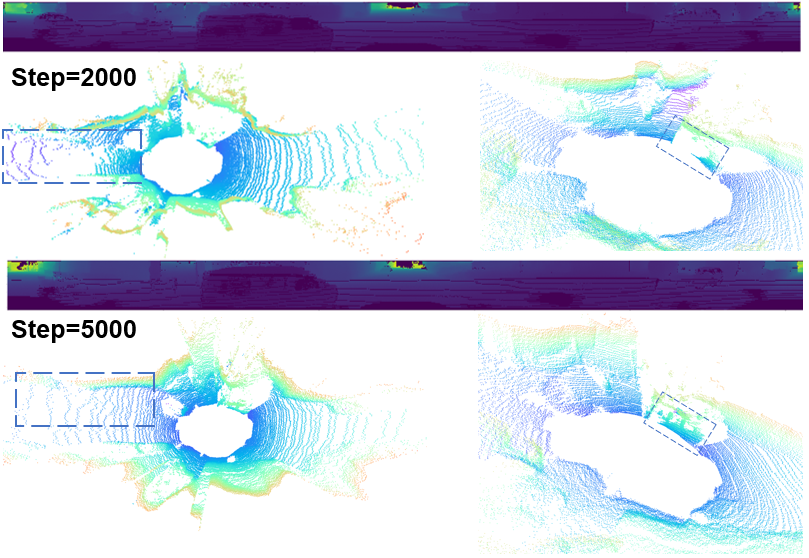}
\caption{Sample Results of LiDARDraft Trained with Different Steps on SemanticKITTI~\cite{behley2019semantickitti}. At 2,000 training steps, the roads have defects, and vehicle details are missing. At 5,000 steps, the roads are smooth, and window details are accurately rendered. With each point cloud input, three generated point clouds samples are presented in the figure. Boxes of the same color correspond to the same scene parts.}
\label{fig:step}
\end{figure}
